# Supplementary material for: Signaling in sensor networks for sequential detection
Source: arXiv:1403.3126 source file (2014-03-12)
Supplement: Supplementary file 1 [file appendix_2_v2.tex]

\section{Proof of Theorem 3}
 \begin{IEEEproof}
  Let \(\Gamma^1=(\gamma^1_1,\gamma^1_2,...,\gamma^1_{T^1})\) be the fixed policy of O1. By definition of \(\pi^2_{k+1}\), we have
   \begin{align}
    &\pi^2_{k+1}(Y^2_{1:k+1},Z^1_{1:k+1}) := P^{\Gamma^1}(H=0|Y^2_{1:k+1},Z^1_{1:k+1}) \nonumber \\
                                            &=P(H=0,Y^2_{k+1},Z^1_{k+1}|Y^2_{1:k},Z^1_{1:k})\nonumber \\ &/\sum_{h=0,1}P(H=h,Y^2_{k+1},Z^1_{k+1}|Y^2_{1:k},Z^1_{1:k})   \label{eq:Apc1}
   \end{align}
   (although we omit the superscript \(\Gamma^1\) for ease of notation, it should be understood that these probabilities are defined with a fixed \(\Gamma^1\)) \\ 
   Consider the numerator in (\ref{eq:Apc1}). It can be written as:
   \begin{align}
   &P(Y^2_{k+1}|H=0,Y^2_{1:k},Z^1_{1:k+1}).P(Z^1_{k+1}|H=0,Y^2_{1:k},Z^1_{1:k}). \nonumber \\&P(H=0|Y^2_{1:k},Z^1_{1:k}) \nonumber \\
   &=P(Y^2_{k+1}|H=0).P(Z^1_{k+1}|H=0,Z^1_{1:k}).\pi^2_k(Y^2_{1:k},Z^1_{1:k}) \label{eq:Apc2}
   \end{align}
   where we used conditional independence of the observations in (\ref{eq:Apc2}). Under a fixed policy of O1, \(Z^1_k\) s are well-defined random variables and hence the second term in (\ref{eq:Apc2}) is well-defined. Similar expressions can be obtained for terms in the denominator of (\ref{eq:Apc1}). Thus, we have that \(\pi^2_{k+1}\) is a function of \(\pi^2_k\), \(Y^2_{k+1}\) and \(Z^1_{1:k+1}\). That is,
   \begin{equation}
    \pi^2_{k+1} = \tilde{T}_k(\pi^2_k,Y^2_{k+1},Z^1_{1:k+1}) \label{eq:Apc2.1}
   \end{equation}
   Also, a fixed policy \(\Gamma^1\) of O1 induces a stopping time function \(S^{\Gamma^1}\) such that
   \begin{equation} \tau^1 = S^{\Gamma^1}(Y^1_{1:T^1}) \end{equation}
   Thus, with a fixed \(\Gamma^1\), the expected delay cost for O1 \((E[c^1\tau^1]\) is fixed and does not depend on the choice of \(\Gamma^2\). 
  Consider any policy \(\Gamma^2\) of O2 and define \(\tilde{W}_k(y^2_{1:k},z^1_{1:k})\) as the expected cost to go for O2 at time \(k\), if O2 has not declared its final decision before time \(k\). That is,
\begin{align}
  \tilde{W}_k(y^2_{1:k},z^1_{1:k}) := E^{\Gamma^1,\Gamma^2}[c^2\tau^2+J(U^2_{\tau^2},H)|y^1_{1:k},z^1_{1:k},U^2_{1:k-1}=N_{1:k-1}]
\end{align}
We will show that these functions are lower bounded by the value functions \(\tilde{V}_k\) defined in the statement of Theorem 3.
   First consider time \(T^2\), we defined \(\tilde{V}_{T^2}\) as
   \begin{align}
  	\tilde{V}_{T^2}(z^1_{1:T^1},\pi) := min \{ &E^{\Gamma^1} [J(0,H)|\pi^2_{T^2}=\pi], \nonumber \\
  	                                  &E^{\Gamma^1} [J(1,H)|\pi^2_{T^2}=\pi]  \} \label{eq:A22.1}
  \end{align}
    
    Now, if O2 has not declared a final decision on the hypothesis till \(T^2-1\), then under policy \(\Gamma^2\), it will either decide \(0\) or \(1\) at time \(T^2\). If O2 selects \(U^2_{T^2} =0\), then his cost to go function at time \(T^2\) is 
    \begin{align}
    &\tilde{W}_{T^2}(y^2_{1:T^2},z^1_{1:T^1}) = \tilde{w}_{T^2}(y^2_{1:T^2},z^1_{1:T^1},0) \nonumber \\ &:=E^{\Gamma^1}[J(0,H)|y^2_{1:T^2},z^1_{1:T^1}] \nonumber \\ = &\pi^2_{T^2}(y^2_{1:T^2},z^1_{1:T^1}).J(0,0) + (1-\pi^2_{T^2}(y^2_{1:T^2},z^1_{1:T^1})).J(0,1) \nonumber \\
    = &E^{\Gamma^1}[J(0,H)|\pi^2_{T^2}(y^2_{1:T^2},z^1_{1:T^1})]
    \end{align}
    Similarly, if O2 selects \(U^2_{T^2} =1\), its cost to go is
    \begin{align}
    &\tilde{W}_{T^2}(y^2_{1:T^2},z^1_{1:T^1}) = \tilde{w}_{T^2}(y^2_{1:T^2},z^1_{1:T^1},1) \nonumber \\ &:=E^{\Gamma^1}[J(1,H)|y^2_{1:T^2},z^1_{1:T^1}] \nonumber \\ = &\pi^2_{T^2}(y^2_{1:T^2},z^1_{1:T^1}).J(1,0) + (1-\pi^2_{T^2}(y^2_{1:T^2},z^1_{1:T^1})).J(1,1) \nonumber \\
    = &E^{\Gamma^1}[J(0,H)|\pi^2_{T^2}(y^2_{1:T^2},z^1_{1:T^1})]
    \end{align} 
    In either case, we have from the definition of \(\tilde{V}_{T^2}\) that
    \[ \tilde{W}_{T^2}(y^2_{1:T^2},z^1_{1:T^1}) \geq \tilde{V}_{T^2}(z^1_{1:T^1},\pi^2_{T^2}(y^2_{1:T^2},z^1_{1:T^1})) \]
    and the optimal action at time \(T^2\) is to select the minimizing option in definition of \(\tilde{V}_{T^2}\). 
    \par
   We will employ backward induction on the functions \(\tilde{V}_k\) defined in Theorem 3 to show that they represent the optimal value functions for O2.  Consider time instant \(k\). Assume \(\tilde{V}_{k+1}\) gives the optimal cost to go function at time \(k+1\). We have,by definition,
   \begin{align}
   &\tilde{V}_k(Z^1_{1:k},\pi) := min \{ \nonumber \\
   &E^{\Gamma^1} [J(0,H)|\pi^2_{k}=\pi], \nonumber \\
  	                                  &E^{\Gamma^1} [J(1,H)|\pi^2_{k}=\pi], \nonumber \\
  	                                  & c^2 + E^{\Gamma^1} [\tilde{V}_{k+1}(Z^1_{1:k+1},\pi^2_{k+1})|\pi^2_{k}=\pi,Z^1_{1:k}]\} \label{eq:A22.2}
  \end{align}
  Then at time \(k\), the cost of stopping and declaring a decision on the hypothesis at time \(k\) is either
    \begin{align}
     \tilde{W}_k(y^2_{1:k},z^1_{1:k}) = E^{\Gamma^1}[J(0,H)|\pi^2_k(y^2_{1:k},z^1_{1:k})] 
   \end{align}   
   or   
    \begin{align}
     \tilde{W}_k(y^2_{1:k},z^1_{1:k}) = E^{\Gamma^1}[J(1,H)|\pi^2_k(y^2_{1:k},z^1_{1:k})] 
   \end{align}   
   By similar arguments as at time \(T^2\), both the above terms are lower bounded by \(\tilde{V}_k(z^1_{1:k},\pi^2_k(y^2_{1:k},z^1_{1:k}))\).
     The cost of continuing at time \(k\) is
     \begin{align}
     &\tilde{W}_k(y^2_{1:k},z^1_{1:k}) = c^2 + E^{\Gamma^1}[\tilde{V}_{k+1}(Z^1_{1:k+1},\pi^2_{k+1})|y^2_{1:k},z^1_{1:k}] \nonumber\\
                                      &= c^2 + \nonumber \\ &E^{\Gamma^1}[\tilde{V}_{k+1}(Z^1_{1:k+1},\tilde{T}_k(\pi^2_k,Y^2_{k+1},Z^1_{1:k+1}))|y^2_{1:k},z^1_{1:k}] \\
                                      &= c^2 + \nonumber \\
                                     &E^{\Gamma^1}[\tilde{V}_{k+1}(z^1_{1:k},Z^1_{k+1},\tilde{T}_k(\pi^2_k,Y^2_{k+1},z^1_{1:k},Z^1_{k+1}))|y^2_{1:k},z^1_{1:k}]  \label{eq:Apc3}
   \end{align}
   The expectation in (\ref{eq:Apc3}) depends on \(\pi^2_k\) and \(P^{\Gamma^1}(Y^2_{k+1},Z^1_{k+1}|y^2_{1:k},z^1_{1:k}) \). This probability can be written as:
   \begin{align}
    &P(Y^2_{k+1}|H=0).P(Z^1_{k+1}|H=0,z^1_{1:k}). \pi^2_k + \nonumber \\&P(Y^2_{k+1}|H=1).P(Z^1_{k+1}|H=1,z^1_{1:k}).(1- \pi^2_k) 
    \end{align}
   which depends only on \(z^1_{1:k}\) and \(\pi^2_k\). Thus, the cost of continuing is
   \[ c^2 + E^{\Gamma^1}[\tilde{V}_{k+1}(Z^1_{1:k+1},\pi^2_{k+1})|\pi^2_k(y^2_{1:k},z^1_{1:k}), z^1_{1:k}] \]
   which corresponds to the last term in the definition of \(\tilde{V}_k\). Thus, \(V_k\) is a lower bound to the expected cost to go for any policy at any time \(k\). Consequently, a policy that always selects the minimizing option in the definition of \(V_k\) achieves the lower bound on the expected cost and is therefore, an optimal policy.
   %Clearly, \(\tilde{V}_k\) now describes the optimal value function.  
\end{IEEEproof}   
   
\section{Proof of Lemma 2}
\begin{IEEEproof}
 The result of Lemma 2 for time \(T^2\) follows from the definition of \(\tilde{V}_{T^2}\) since
 \[E^{\Gamma^1} [J(0,H)|\pi^2_{T^2}=\pi] = \pi.J(0,0) + (1-\pi).J(0,1)  \]
 This corresponds to the line \(l^0(\pi)\). Similarly,
 \[E^{\Gamma^1} [J(1,H)|\pi^2_{T^2}=\pi] = \pi.J(1,0) + (1-\pi).J(1,1)  \]
 which corresponds to line \(l^1(\pi)\).
Since, for any realization of \(z^1_{1:T^1}\), \(\tilde{V}_{T^2}\) is minimum of two affine functions of \(\pi\), it is concave in \(\pi\) for each \(z^1_{1:T^1}\).  
\par
Assume now that \(\tilde{V}_{k+1}(z^1_{1:k+1},\pi)\) is concave in \(\pi\) for each \(z^1_{1:k+1}\). Then, we can write \(\tilde{V}_{k+1}\) as:
 \begin{equation} \label{eq:Apinfimum2}
 \tilde{V}_{k+1}(z^1_{1:k+1},\pi) = \inf_i \{ \lambda_i(z^1_{1:k+1}).\pi + \mu_i(z^1_{1:k+1}) \} \end{equation}
 
 where \(\lambda_i(z^1_{1:k+1})\) and \(\mu_i(z^1_{1:k+1}) \) are real numbers that depend on \(z^1_{1:k+1}\).
 Consider the value-function at time \(k\).
 \begin{align}
   \tilde{V}_k(z^1_{1:k},\pi) = min \{&E^{\Gamma^1} [J(0,H)|\pi^2_{k}=\pi], \nonumber \\
  	                                  &E^{\Gamma^1} [J(1,H)|\pi^2_{k}=\pi], \nonumber \\
  	                                  & c^2 + E^{\Gamma^1} [\tilde{V}_{k+1}(Z^1_{1:k+1},\pi^2_{k+1})|\pi^2_{k}=\pi,z^1_{1:k}]\}  \label{eq:Apd1}
  \end{align}
  The first two terms in (\ref{eq:Apd1}) correspond to the affine terms \(l^0\) and \(l^1\). The last term in (\ref{eq:Apd1}) can be written as:
  \begin{align}
  &c^2 + E^{\Gamma^1} [\tilde{V}_{k+1}(Z^1_{1:k+1},\pi^2_{k+1})|\pi^2_{k}=\pi,z^1_{1:k}]\}  \nonumber \\
  = &c^2 + E^{\Gamma^1} [\tilde{V}_{k+1}(Z^1_{1:k+1},\tilde{T}_k(\pi^2_k,Y^2_{k+1},Z^1_{1:k+1}))|\pi^2_{k}=\pi,z^1_{1:k}]\}  \nonumber \\
  = &c^2 + \sum\limits_{y^2_{k+1} \in \mathcal{Y}^2} \sum\limits_{z^1_{k+1} \in \{0,1,b\}} [Pr(y^2_{k+1},z^1_{k+1}|\pi^2_k=\pi,z^1_{1:k}). \nonumber \\ &\tilde{V}_{k+1}(z^1_{1:k+1},\tilde{T}_k(\pi,y^2_{k+1},z^1_{1:k+1})) ]  \label{eq:Apd2}	
  \end{align}
  We now use the fact that \(\tilde{T}_k(\pi,y^2_{k+1},z^1_{1:k+1})\) is given as
  \begin{align}
  &P(y^2_{k+1}|H=0).P(z^1_{k+1}|H=0,z^1_{1:k}).\pi/ \nonumber \\&P(y^2_{k+1},z^1_{k+1}|\pi^2_k=\pi,z^1_{1:k})
  \end{align}
 
  Focusing on one term of the summation in (\ref{eq:Apd2}) and using (\ref{eq:Apinfimum2}), we can write it as
  \begin{align}
     &P(y^2_{k+1},z^1_{k+1}|\pi^2_k=\pi,z^1_{1:k}) \times \nonumber \\ &\inf_i\{\lambda_i(z^1_{1:k+1}).(P(y^2_{k+1}|H=0).P(z^1_{k+1}|H=0,z^1_{1:k}).\pi/ \nonumber \\ &P(y^2_{k+1},z^1_{k+1}|\pi^2_k=\pi,z^1_{1:k})) + \mu_i(z^1_{1:k+1}) \} \label{eq:Apd3}
  \end{align}
  
  Note that the expression outside the infimum in (\ref{eq:Apd3}) is same as the denominator in the term multiplying \(\lambda_i(z^1_{1:k+1})\) in (\ref{eq:Apd3}). Equation  (\ref{eq:Apd3}) can now be expressed as
  \begin{align}
  &\inf_i\{\lambda_i(z^1_{1:k+1}).P(y^2_{k+1}|H=0).P(z^1_{k+1}|H=0,z^1_{1:k}).\pi \nonumber \\
 +&\mu_i(z^1_{1:k+1}). P(y^2_{k+1},z^1_{k+1}|\pi^2_k=\pi,z^1_{1:k}) \label{eq:Ape.1}
 \end{align}
   Now expanding the probability multiplying \(\mu_i\), we get
   \begin{align}
 &\inf_i\{\lambda_i(z^1_{1:k+1}).P(y^2_{k+1}|H=0).P(z^1_{k+1}|H=0,z^1_{1:k}).\pi \nonumber \\ +&\mu_i(z^1_{1:k+1}).(P(y^2_{k+1}|H=0).P(z^1_{k+1}|H=0,z^1_{1:k}).\pi + \nonumber \\ &P(y^2_{k+1}|H=1).P(z^1_{k+1}|H=1,z^1_{1:k}).(1-\pi)) \}  \label{eq:Apd5}
  \end{align} 
 For the given \(z^1_{1:k+1}\) and \(y^2_{k+1}\), the term in the infimum in (\ref{eq:Apd5}) is affine in \(\pi\). Therefore, the expression in (\ref{eq:Apd5}) is concave in \(\pi\). Thus each term in the summation in (\ref{eq:Apd2}) is concave in \(\pi\) for the given realization of \(z^1_{1:k}\). Hence, the sum is concave in \(\pi\) as well. This establishes the structure of \(\tilde{V}_k\) in Lemma 2. To complete the induction argument, we only have to note that since \(\tilde{V}_k\) is the minimum of 2 affine and one concave function of \(\pi\) , it is concave in \(\pi\) (for each \(z^1_{1:k}\)).
 \end{IEEEproof}
