# Supplementary material for: Signaling in sensor networks for sequential detection
Source: arXiv:1403.3126 source file (2014-03-12)
Supplement: Supplementary file 2 [file mtns_appendix.tex]

\appendices

 \section{Proof of Lemma 1} \label{sec:lemma_1}
 \begin{proof}
 Part (i) follows from definition of $\tau^1$.
  
 In Part (ii), if $\tau^1 < t$, then by definition, we have 
 \begin{align} \Pi^2_t &:= P(H=0|Y^2_{1:t},U^1_{1:t-1},U^2_{1:t-1}=b_{1:t-1}) \notag \\
 &= P(H=0|Y^2_{1:t},U^1_{1:\tau^1}) \label{eq:mtnsapp1.4}
  \end{align}
 where we removed redundant terms from the conditioning (terms which are constants or functions of other terms).
 Similarly, 
 \begin{align} \Pi^2_{t+1} =  P(H=0|Y^2_{1:t+1},U^1_{1:\tau^1}), \notag  
 \end{align}
 which, on using Bayes' rule gives,
 \begin{align}
   \Pi^2_{t+1}&= \frac{P(Y^2_{t+1}|H=0)\Pi^2_t}{P(Y^2_{t+1}|H=0)\Pi^2_t + P(Y^2_{t+1}|H=1)(1-\Pi^2_t)} \notag \\
   &=: f_{t+1}(\Pi^2_{t+1},Y^2_{t+1})\label{eq:Ap1}
 \end{align}
 
 If $\tau^1 \geq t$, then $U^1_{1:t-1}=b_{1:t-1}$ (that is all decisions of observer 1 are blanks till time $t-1$) and
 \begin{align} \Pi^2_{t} &:= P(H=0|Y^2_{1:t},U^1_{1:t-1}=b_{1:t-1},U^2_{1:t-1}=b_{1:t-1}) \notag 
 \end{align}
 Also,
 %Also, since $t < \tau^2$, $U^2_{1:t}=b_{1:t}$
 \begin{align} &\Pi^2_{t+1} := P(H=0|Y^2_{1:t+1},U^1_{1:t-1}=b_{1:t-1},U^1_t,U^2_{1:t}=b_{1:t}) \notag \\
 %&= P(H=0|Y^2_{1:t+1},U^1_{1:t-1}=b_{1:t-1},U^1_t), \label{eq:mtnsapp1.2}
%\end{align}
%where we included $U^2_{1:t}=b_{1:t}$ in the conditioning in (\ref{eq:mtnsapp1.2}) since it is a function of terms already in the conditioning. Further, using Bayes' rule, we can write (\ref{eq:mtnsapp1.2}) as
%\begin{align} 
 &=\frac{P(Y^2_{t+1},U^1_t,H=0|Y^2_{1:t},U^1_{1:t-1}=b_{1:t-1},U^2_{1:t}=b_{1:t})}{\displaystyle\sum_{h\in \{0,1\}}P(Y^2_{t+1},U^1_t,h|Y^2_{1:t},U^1_{1:t-1}=b_{1:t-1},U^2_{1:t}=b_{1:t})} \label{eq:mtnsapp1.1}
 \end{align}
 The numerator in (\ref{eq:mtnsapp1.1}) can be written as:
 \begin{align}
 &P(Y^2_{t+1}|H=0)\cdot \notag \\&\{P(U^1_t|H=0,Y^2_{1:t},U^1_{1:t-1}=b_{1:t-1},U^2_{1:t}=b_{1:t})\}\Pi^2_t \label{eq:mtnsapp1.3}
 %=&P(Y^2_{t+1}|H=0)\cdot\notag\\&\{P(U^1_t|H=0,U^1_{1:t-1}=b_{1:t-1},U^2_{1:t}=b_{1:t})\}\Pi^2_t 
 \end{align}
  
 We now focus on the second term in (\ref{eq:mtnsapp1.3}).\\
 \emph{Claim:} Consider a realization $u^1_t$, $y^2_{1:t}$. Then, 
 \begin{align}
 &P(u^1_t|H=0,y^2_{1:t},U^1_{1:t-1}=b_{1:t-1},U^2_{1:t}=b_{1:t}) \notag \\
 &= P(u^1_t|H=0,U^1_{1:t-1}=b_{1:t-1},U^2_{1:t}=b_{1:t}) \label{eq:mtnsapp1.7}
 \end{align}
 Moreover, under the given choice of $\Gamma^1$, the probability on the right hand side of (\ref{eq:mtnsapp1.7}) is a function only of $u^1_t$.
 \par
 \emph{Proof of claim:} Using Bayes' rule,
 \begin{align}
 &P(u^1_t|H=0,y^2_{1:t},U^1_{1:t-1}=b_{1:t-1},U^2_{1:t}=b_{1:t}) \notag \\
 &= \frac{P(u^1_t,H=0,y^2_{1:t},U^1_{1:t-1}=b_{1:t-1},U^2_{1:t}=b_{1:t})}{\displaystyle\sum_{u'}P(U^1_t=u',H=0,y^2_{1:t},U^1_{1:t-1}=b_{1:t-1},U^2_{1:t}=b_{1:t})} \label{eq:mtnsapp1.10}
 \end{align}
 Consider the joint probability in the numerator in (\ref{eq:mtnsapp1.10})
 \begin{align}
 P(u^1_t,H=0,y^2_{1:t},b^1_{1:t-1},b^2_{1:t}) \notag 
 \end{align}
 where we use $b^1_{1:t-1},b^2_{1:t-1}$ as shorthand notations for  $U^1_{1:t-1}=b_{1:t-1}$ and $U^2_{1:t-1}=b_{1:t-1}$ respectively. This probability can be further written as:  
 \begin{align}
 &=\displaystyle\sum_{y^1_{1:t}}P(u^1_t,H=0,y^2_{1:t},b^1_{1:t-1},b^2_{1:t},y^1_{1:t}) \notag\\ 
 &=\displaystyle\sum_{y^1_{1:t}}[ P(u^1_t|y^1_{1:t},b^1_{1:t-1},b^2_{1:t-1})\notag\\&\cdot P(U^2_t=b|y^2_{1:t},b^1_{1:t-1},b^2_{1:t-1}) \notag\\
 &\cdot P(y^1_t|H=0)P(y^2_t|H=0)\notag\\ &\cdot \displaystyle\prod_{k=1}^{t-1}\{P(U^1_k=b|y^1_{1:k},b^1_{1:k-1},b^2_{1:k-1})\notag\\&\cdot P(U^2_k=b|y^2_{1:k},b^1_{1:k-1},b^2_{1:k-1}) \notag\\&\cdot P(y^1_k|H=0)P(y^2_k|H=0)\} ] \cdot p_0 \label{eq:mtnsapp1.5}
 \end{align}
 %\begin{align}
 Rearranging the summation in (\ref{eq:mtnsapp1.5}), we get
 \begin{align}
 &P(U^2_t=b|y^2_{1:t},b^1_{1:t-1},b^2_{1:t-1})P(y^2_t|H=0) \cdot p_0 \notag\\
 &\cdot\displaystyle\prod_{k=1}^{t-1}\{P(U^2_k=b|y^2_{1:k},b^1_{1:k-1},b^2_{1:k-1}) P(y^2_k|H=0)\} \notag \\
 &\cdot\displaystyle\sum_{y^1_{1:t}}[ P(u^1_t|y^1_{1:t},b^1_{1:t-1},b^2_{1:t-1})P(y^1_t|H=0)\notag\\ &\cdot \displaystyle\prod_{k=1}^{t-1}\{P(U^1_k=b|y^1_{1:k},b^1_{1:k-1},b^2_{1:k-1}) P(y^1_k|H=0)\} ]  \label{eq:mtnsapp1.6}
 \end{align}
 Expressions similar to (\ref{eq:mtnsapp1.6}) hold for each term in the denominator of (\ref{eq:mtnsapp1.10}) and the terms outside the summation over $y^1_{1:t}$ cancel out in the numerator and the denominator. We note that the summation over $y^1_{1:t}$ in (\ref{eq:mtnsapp1.6}) does not depend on $y^2_{1:t}$. Hence, the conditional probability in the left hand side of (\ref{eq:mtnsapp1.10}) does not depend on $y^2_{1:t}$. This establishes equation (\ref{eq:mtnsapp1.7}). We also note that under the fixed policy $\Gamma^1$ of observer~1, the summation over $y^1_{1:t}$ in (\ref{eq:mtnsapp1.6}) is a function only of $u^1_t$. Thus, the probability on the right hand side of (\ref{eq:mtnsapp1.7}) is a function only of $u^1_t$. This concludes the proof of the claim.
\par
 
Using the result of the claim in (\ref{eq:mtnsapp1.3}) and using similar arguments for the denominator in (\ref{eq:mtnsapp1.1}), we get  
 \begin{align} &\Pi^2_{t+1} \notag\\
 &=\frac{P(Y^2_{t+1}|H=0)P(U^1_t|H=0,b^1_{1:t-1},b^2_{1:t})\Pi^2_t}{\begin{array}{l}P(Y^2_{t+1}|H=0)P(U^1_t|H=0,b^1_{1:t-1},b^2_{1:t})\Pi^2_t \\ +P(Y^2_{t+1}|H=1)P(U^1_t|H=1,b^1_{1:t-1},b^2_{1:t})(1-\Pi^2_t) \end{array} } \notag \\
 &=: g_{t+1}(\Pi^2_{t+1},Y^2_{t+1},U^1_t) \label{eq:g_def}
 \end{align}
 \end{proof}
