# Supplementary material for: Signaling in sensor networks for sequential detection
Source: arXiv:1403.3126 source file (2014-03-12)
Supplement: Supplementary file 3 [file mtns_appendix_part2_versionB.tex]

\section{Proof Outline of Theorem 1}\label{sec:info_states_proof}
%\todo {1. Outline of Theorem 1 proof}
We provide an outline of the proof of Theorem~1. The general idea is to show that at each time $t$, the value functions of Definition~2 represent the optimal future costs. Therefore, a policy that for each realization of $\Pi^2_t, \ind_{\{\tau^1<t\}}$ selects the minimizing term in the corresponding value function achieves the optimal cost. Thus, an optimal policy can be found that depends only on $\Pi^2_t, \ind_{\{\tau^1<t\}}$. We start from time $T$.

\par
 If the observer~2 is active at the terminal time $T$, it can only make one of two decisions: $0$ or $1$. The expected future cost of choosing $u \in \{0,1\}$ for observer~2 is
\begin{align}
&E[J(u,H)|Y^2_{1:T},U^1_{1:T-1},U^2_{1:T-1}=b_{1:T-1}] \notag \\
&=  J(u,0)\Pi^2_T + J(u,1)(1-\Pi^2_T)\notag\\
&= E[J(u,H)|\Pi^2_{T}] \label{eq:app2.2}
\end{align}
Thus, the value function at time $T$ is the minimum of the expected future costs incurred by choosing $0$ or $1$. Hence, it represents the optimal expected future cost for observer~2 at time $T$. Proceeding backwards, we assume that the value functions at time $t+1,t+2,\ldots,T$ represent optimal future costs at the respective times and consider two cases at each time $t<T$. 
\medskip

\emph{Case A: $\tau^1<t$} If observer~1 has already stopped before $t$, then observer~2's stopping problem is the same as the centralized Wald problem and the value function $V_t(\pi,1)$ is same as the value function in the dynamic program for the Wald problem.

\emph{Case B: $\tau^1 \geq t$} We now consider the case when observer~1 has not stopped before time $t$. If observer~2 decides to stop and chooses $u \in \{0,1\}$ at time $t$, then the expected future cost will be
\begin{align}
 \mathds{E}\Big[&\ind_{\{\tau^1=t\}}J(u,H) \notag \\&+ \ind_{\{\tau^1>t\}}(k(\tau^1-t)+ J(U^1_{\tau^1},H))\bigg|\begin{array}{l}Y^2_{1:t},b^1_{1:t-1}\\,b^2_{1:t-1},U^2_t=u \end{array}\Big] \label{eq:app2.1}
\end{align}

\emph{Claim:} The expectation in (\ref{eq:app2.1}) is same as:
\begin{align}
&\mathds{E}[\ind_{\{\tau^1=t\}}J(u,H) + \notag \\&\ind_{\{\tau^1>t\}}(k(\tau^1-t)+ J(U^1_{\tau^1},H))|\Pi^2_t,\ind_{\{\tau^1<t\}}=0,U^2_t=u]
\end{align}
\emph{Proof of claim:}
For each realization $y^2_{1:t}$ of observer~2's observations, the expectation in (\ref{eq:app2.1}) depends on the conditional distribution of the following random variables: $H,\tau^1,U^1_{\tau^1}$ given the realization of the random variables $y^2_{1:t},b^1_{1:t-1},b^2_{1:t-1},U^2_t=u$. Note that under the fixed policy $\Gamma^1$ of observer~1, $\tau^1,U^1_{\tau^1}$ are functions of observer~1's observation sequence $Y^1_{1:T}$ and the terms $b^1_{1:t-1},b^2_{1:t-1},U^2_t=u$ fixed in the conditioning.  Hence the conditional belief
\[ P(H,\tau^1,U^1_{\tau^1}|y^2_{1:t},b^1_{1:t-1},b^2_{1:t-1},U^2_t=u) \]
is a deterministic transformation of the belief
\[ P(H,Y^1_{1:T}|y^2_{1:t},b^1_{1:t-1},b^2_{1:t-1},U^2_t=u).\]
We will show that the above probability is same as 
\[ P(H,Y^1_{1:T}|\pi^2_t,\ind_{\{\tau^1<t\}} =0,U^2_t=u)\]
and hence the conditional expectation in (\ref{eq:app2.1}) is same as 
\begin{align*} \mathds{E}[&\ind_{\{\tau^1=t\}}J(u,H)+ \notag \\&\ind_{\{\tau^1>t\}}(k(\tau^1-t)+ J(U^1_{\tau^1},H))|\pi^2_{t},\ind_{\{\tau^1<t\}=0},U^2_t=u]\end{align*}
which corresponds to the first two terms in the minimization in $V_t(\pi^2_t,0)$ in equation (\ref{eq:defv0}).

Consider $P(H=0,y^1_{1:T}|y^2_{1:t},b^1_{1:t-1},b^2_{1:t-1},U^2_t=u)$
\begin{align}
&=P(y^1_{1:T}|H=0,y^2_{1:t},b^1_{1:t-1},b^2_{1:t-1},U^2_t=u)\pi^2_t \label{eq:app2.5} 
\end{align}
Similarly, 
\begin{align}
&P(H=0,y^1_{1:T}|\pi^2_t,\ind_{\{\tau^1<t\}}=0,U^2_t=u) \notag \\
&= P(y^1_{1:T}|H=0,\pi^2_t,\ind_{\{\tau^1<t\}}=0,U^2_t=u)\pi^2_t \label{eq:app2.6}
\end{align}
We now compare the first terms in (\ref{eq:app2.5}) and (\ref{eq:app2.6}). Consider the first term in (\ref{eq:app2.5}), which can be written as
\begin{align}
&= \frac{P(H=0,y^1_{1:T},y^2_{1:t},b^1_{1:t-1},b^2_{1:t-1},U^2_t=u)}{\displaystyle\sum_{\tilde{y}^1_{1:T}} P(H=0,\tilde{y}^1_{1:T},y^2_{1:t},b^1_{1:t-1},b^2_{1:t-1},U^2_t=u)} \label{eq:app2.3}
\end{align}
The numerator can be written as:
\begin{align}
 &P(y^1_{t+1:T}|H=0)P(U^2_t=u|y^2_{1:t},b^1_{1:t-1},b^2_{1:t-1}) \notag\\
 &\cdot P(y^1_t|H=0)P(y^2_t|H=0)\notag\\ &\cdot \displaystyle\prod_{k=1}^{t-1}\{P(U^1_k=b|y^1_{1:k},b^1_{1:k-1},b^2_{1:k-1})\notag\\&\cdot P(U^2_k=b|y^2_{1:k},b^1_{1:k-1},b^2_{1:k-1}) \notag\\&\cdot P(y^1_k|H=h)P(y^2_k|H=h)\} \cdot p_0
\end{align}
Similar expressions hold for the denominator in (\ref{eq:app2.3}) and the terms that depend on $y^2_{1:t}$ will cancel in the numerator and the denominator. Therefore,
\begin{align}
&P(y^1_{1:T}|H=0,y^2_{1:t},b^1_{1:t-1},b^2_{1:t-1},U^2_t=u) \notag\\
&= P(y^1_{1:T}|H=0,b^1_{1:t-1},b^2_{1:t-1},U^2_t=u)\label{eq:app2.7} 
%&= P(y^1_{1:T}|H=0,\ind_{\{\tau^1<t\}}=0,U^2_t=u) 
\end{align}
Now consider the first term in (\ref{eq:app2.6}) which can be written as:
\begin{align}
&P(y^1_{1:T}|H=0,\pi^2_t,\ind_{\{\tau^1<t\}}=0,U^2_t=u) \notag\\
&=\displaystyle \sum_{y^2_{1:t}}[P(y^1_{1:T}|y^2_{1:t},H=0,\pi^2_t,\ind_{\{\tau^1<t\}}=0,U^2_t=u) \notag\\
&\cdot P(y^2_{1:t}|H=0,\pi^2_t,\ind_{\{\tau^1<t\}}=0,U^2_t=u)] \notag \\
&= \displaystyle \sum_{y^2_{1:t}}[P(y^1_{1:T}|y^2_{1:t},H=0,b^1_{1:t-1},b^2_{1:t-1},U^2_t=u) \notag\\
&\cdot P(y^2_{1:t}|H=0,\pi^2_t,\ind_{\{\tau^1<t\}}=0,U^2_t=u)] \label{eq:neweq1}
\end{align}
The first term inside the summation in (\ref{eq:neweq1}) is same as LHS of (\ref{eq:app2.7}). Using (\ref{eq:app2.7}) in (\ref{eq:neweq1}) gives
\begin{align}
& \displaystyle \sum_{y^2_{1:t}}[P(y^1_{1:T}|H=0,b^1_{1:t-1},b^2_{1:t-1},U^2_t=u) \notag\\
&\cdot P(y^2_{1:t}|H=0,\pi^2_t,\ind_{\{\tau^1<t\}}=0,U^2_t=u)] \notag \\
&= P(y^1_{1:T}|H=0,b^1_{1:t-1},b^2_{1:t-1},U^2_t=u) \label{eq:app2.8}
\end{align} 
which is same as RHS of (\ref{eq:app2.7}). Thus the probabilities in RHS of (\ref{eq:app2.5}) and (\ref{eq:app2.6}) are equal. This implies the equality of expectations and completes the proof of the claim.
\par
As a consequence of the claim, the first two terms in the minimization in the definition of $V_t(\pi,0)$ (equation \ref{eq:defv0}) correspond to the expected future cost of choosing $0$ or $1$ at time $t$. On the other hand, if observer~2 decides to continue at time $t$, then by the fact that value functions at $t+1$ represent the expected future costs at $t+1$, we can write the expected future cost as:
\begin{align}
&\mathds{E}\Big[\ind_{\{\tau^1=t\}}(k+V_{t+1}(\Pi_{t+1},1)) \nonumber \\
 &~~+\ind_{\{\tau^1>t\}}(K+V_{t+1}(\Pi_{t+1},0))\bigg|\begin{array}{l}Y^2_{1:t},b^1_{1:t-1}\\,b^2_{1:t-1},U^2_t=b \end{array}\Big] \label{eq:app2.1.B}
\end{align}

Using lemma 1 and the fact that under fixed policy $\Gamma^1$ of observer~1, $U^1_{t}$ is a function of observer~1's observation sequence $Y^1_{1:t}$ and the terms $b^1_{1:t-1},b^2_{1:t-1}$ fixed in the conditioning , one can conclude that for each realization of $y^2_{1:t}$ this expectation in (\ref{eq:app2.1.B}) is a function of the following conditional probability:\[P(Y^1_{1:t},Y^2_{t+1}|y^2_{1:t},b^1_{1:t-1},b^2_{1:t-1},U^2_t=b)\]
Using arguments similar to those in the claim above, it can be shown that the above conditional probability is same as:
\[ P(Y^1_{1:t},Y^2_{t+1}|\pi^2_t,\ind_{\{\tau^1<t\}} =0,U^2_t=b)\]
This shows that the third term in the minimization in the definition of $V_t(\pi,0)$ (equation \ref{eq:defv0}) is the expected future cost of making a decision to continue at time $t$. Thus,
$V_t(\Pi^2_t,0)$ is the minimum of the future costs incurred by choosing $0,1$ or $b$. Hence, it represents the optimal future cost at time $t$, if observer~1 has not already stopped before time $t$.

\section{Proof Outline of Lemma 2} \label{sec:lemma_2}
 We define the following functions
 \begin{align*}
 l^0(\pi) :&= J(0,0)\pi+J(0,1)(1-\pi) \notag\\
 &=\mathds{E}[J(0,H)|\Pi^2_t =\pi] \\
  l^1(\pi) :&= J(1,0)\pi+J(1,1)(1-\pi) \notag\\
 &=\mathds{E}[J(1,H)|\Pi^2_t =\pi]
 \end{align*} 
 For the value function at time $T$, the result of the lemma follows from the definitions of $l^0(\pi), l^1(\pi)$ and $V_T(\pi,a)$. Since, for each $a \in \{0,1\}$, $V_T(\pi,a)$ is the minimum of two affine functions of $\pi$, it implies that, for each $a \in \{0,1\}$, $V_T(\pi,a)$ is a concave function of $\pi$. Now, assume that $V_{t+1}(\pi,a)$ is concave in $\pi$ for each $a \in \{0,1\}$. The concavity of the value functions at time $t+1$ implies that they can be written as infimum of affine functions of $\pi$. In particular, we have
 \begin{align} \label{eq:concave_1}
 V_{t+1}(\pi,1) = \inf_{i}\{ a_i\pi+b_i\}
 \end{align} 
 and 
\begin{align} \label{eq:concave_2}
 V_{t+1}(\pi,0) = \inf_{i} \{c_i\pi+d_i\}
 \end{align}
 Now consider $V_t(\pi,1)$. The first two terms in the definition of $V_t(\pi,1)$ are affine in $\pi$ (see Definition 2). We need to show that the third term -
 \begin{equation} \label{eq:app3.1}
 k+ \mathds{E}[V_{t+1}(\Pi^2_{t+1},1)|\Pi^2_{t}=\pi,\ind_{\{\tau^1<t\}=1}] \end{equation}
 -is a concave function of $\pi$. From equation (\ref{eq:Ap1}) in the proof of lemma 1, we know that $\Pi_{t+1}$ can be written as:
 \begin{align}
 \Pi^2_{t+1}&= \frac{P(Y^2_{t+1}|H=0)\Pi^2_t}{P(Y^2_{t+1}|H=0)\Pi^2_t + P(Y^2_{t+1}|H=1)(1-\Pi^2_t)} \notag \\
            &= \frac{P(Y^2_{t+1}|H=0)\Pi^2_t}{P(Y^2_{t+1}|\Pi^2_t)}  \label{eq:app3.2}
 \end{align}
 Substituting (\ref{eq:app3.2}) in (\ref{eq:app3.1}) and evaluating the expectation gives:
 \begin{align}
  k + \displaystyle\sum_{y \in \mathcal{Y}}&P(Y^2_{t+1}=y|\Pi^2_{t}=\pi,\ind_{\{\tau^1<t\}}=1) \notag\\
                                           &V_{t+1}\left(\frac{P(Y^2_{t+1}=y|H=0)\pi}{P(Y^2_{t+1}=y|\pi)},1\right) 
 \end{align}
 Now using the characterization of $V_{t+1}(\pi,1)$ from (\ref{eq:concave_1}), we get
 \begin{align}
  k + \displaystyle\sum_{y \in \mathcal{Y}}&P(Y^2_{t+1}=y|\Pi^2_{t}=\pi) \notag\\
                                           &\left[ \inf_i\{ a_i\left(\frac{P(Y^2_{t+1}=y|H=0)\pi}{P(Y^2_{t+1}=y|\pi)}\right) +b_i \} \right] \notag\\
  =k + \displaystyle\sum_{y \in \mathcal{Y}}  & \inf_i \{ a_i(P(Y^2_{t+1}=y|H=0)\pi) \notag \\&+b_iP(Y^2_{t+1}=y|H=0)\pi\notag\\&+ b_iP(Y^2_{t+1}=y|H=1)(1-\pi) \}                                \end{align}
 Each term in the summation over $y \in \mathcal{Y}$ is infimum of affine functions of $\pi$, hence each term in the summation is a concave function of $\pi$. Thus,  the third term of $V_t(\pi,1)$ is a concave function of $\pi$.
  
  \par
  Next consider $V_t(\pi,0)$ defined in (\ref{eq:defv0}). The conditional expectation for the first (or second) term in the minimization in RHS of (\ref{eq:defv0}) is an affine function of the conditional probability of the random variables $H, Y^1_{1:T}$. Using arguments from Appendix~\ref{sec:info_states_proof}, this conditional probability can be written as:
  \begin{align}
  &P(y^1_{1:T},H=0|\pi^2_t,b^1_{1:t-1},b^2_{1:t-1},U^2_t=0) \notag \\
  &= P(y^1_{1:T}|H=0,b^1_{1:t-1},b^2_{1:t-1},U^2_t=0)\pi^2_t
 \end{align}
  and
  \begin{align}
  &P(y^1_{1:T},H=1|\pi^2_t,b^1_{1:t-1},b^2_{1:t-1},U^2_t=0) \notag \\
  &= P(y^1_{1:T}|H=1,b^1_{1:t-1},b^2_{1:t-1},U^2_t=0)(1-\pi^2_t)
 \end{align}
 Thus, the conditional probability $P(Y^1_{1:T},H|\pi^2_t,b^1_{1:t-1},b^2_{1:t-1},U^2_t=0)$ is an affine function of $\pi^2_t$. This establishes the affine nature of the first two terms of RHS of (\ref{eq:defv0}) . The third term in $V_t(\pi,0)$ can be written as:
 \begin{align}
 &\mathds{E}\Big[\ind_{\{U^1_t \neq b\}}(k+V_{t+1}(g_{t+1}(\pi,Y^2_{t+1},U^1_t),1)) \nonumber \\
 &+\ind_{\{U^1_t=b\}}(K+V_{t+1}(g_{t+1}(\pi,Y^2_{t+1},b),0))\Big|\begin{array}{l}\Pi^2_{t}=\pi,\\\ind_{\{\tau^1<t\}=0},\\U^2_t=b\end{array}\Big] \label{eq:app3.3}
 \end{align}
 Consider the first term in the summation in (\ref{eq:app3.3}). Evaluating the expectation and using the characterization of $g_{t+1}$ from (\ref{eq:mtnsapp1.1}) and (\ref{eq:g_def}), we get
 \begin{align}
 &\displaystyle \sum_{u^1_t,y^2_{t+1}} [\ind_{\{u^1_t \neq b\}}(k+V_{t+1}(g_{t+1}(\pi,y^2_{t+1},u^1_t),1)) \notag \\ &\cdot P(u^1_t,y^2_{t+1}|\Pi^2_{t}=\pi,\ind_{\{\tau^1<t\}=0},U^2_t=b)]\notag\\
 &=\displaystyle \sum_{u^1_t,y^2_{t+1}} [\ind_{\{u^1_t \neq b\}}(k+ \notag\\&V_{t+1}\left(\frac{P(y^2_{t+1}|H=0)P(u^1_t|H=0,b^1_{1:t-1},b^2_{1:t})\pi}{P(y^2_{t+1},u^1_t|\Pi^2_t=\pi,b^1_{1:t-1},b^2_{1:t})},1\right))] \notag\\
 &\cdot P(u^1_t,y^2_{t+1}|\Pi^2_{t}=\pi,\ind_{\{\tau^1<t\}=0},U^2_t=b)]\label{eq:app3.4} 
 \end{align}
 Using the characterization of $V_{t+1}(\pi,1)$ from (\ref{eq:concave_2})  in (\ref{eq:app3.4}), we get
 \begin{align}
 &\displaystyle \sum_{u^1_t=0,1}\displaystyle \sum_{y^2_{t+1}}[k \notag\\&+ \inf_i \{ c_iP(y^2_{t+1}|H=0)P(u^1_t|H=0,b^1_{1:t-1},b^2_{1:t})\pi \notag \\
 &+d_iP(y^2_{t+1}|H=0)P(u^1_t|H=0,b^1_{1:t-1},b^2_{1:t})\pi \notag\\&+ d_iP(y^2_{t+1}|H=1)P(u^1_t|H=1,b^1_{1:t-1},b^2_{1:t})(1-\pi)\}]
 \end{align}
 which is concave in $\pi$ (since it is infimum of affine functions in $\pi$). Similar arguments can be made for the second term in (\ref{eq:app3.3}) to conclude the concavity of third term in $V_t(\pi,0)$.
